# Supplementary material for: Modeling electrochemical systems with weakly imposed Dirichlet boundary conditions
Source: arXiv:2010.08778 source file (2021-08-22)
Supplement: Supplementary file 1 [file table.tex]

\begin{landscape}
\begin{table}[h] 
\centering
\begin{tabular}{c c c c}
\toprule % Top horizontal line
\textbf{Characteristic} & \multicolumn{1}{c}{\textbf{Non-dimensional}}  
& \multicolumn{1}{c}{\textbf{Non-dimensional}} 
    & \textbf{\(\kappa\)} \\
\textbf{variables} & \textbf{numbers} & \textbf{equations} \\
\cmidrule{1-4}\morecmidrules\cmidrule{1-4}
%\cmidrule(1){1-4}\morecmidrules\cmidrule(1){1-4} % Horizontal line spanning less than the full width of the
\(U_{ref} = U\) & \(Pe=\frac{UL}{D}\) & \(\frac{dc_{i}}{dt} + \vec{u} \cdot \nabla c_{i}
                        = \frac{1}{Pe}\nabla \cdot (\nabla c_{i} 
                    + z_{i} c_{i}\nabla \phi)\) &  \\
\(t_{ref}=L/U\) &\(\Lambda=\frac{\lambda}{L}\)  & \(-2 \Lambda^2 \nabla^2\phi = \Sigma c_i z_i\) & \(\frac{\varepsilon}{\eta LU} \left (\frac{RT}{F}\right)^2\)\\
\(p_{ref} = \eta U/L \) & \(Re=\frac{\rho UL}{\eta}\) & \( Re \frac{d\vec{u}}{dt} + Re \: \vec{u}\cdot\nabla\vec{u}
                            =- \nabla p + \nabla^{2}\vec{u} - 
                            \frac{\kappa}{2\Lambda^2} \Sigma c_i z_i\nabla \phi\)\ &  \\
                            
\cmidrule(l){1-4} % Horizontal line spanning less than the full width of the

\(U_{ref} = U\) & \(Pe=\frac{UL}{D}\) & \(\frac{dc_{i}}{dt} + \vec{u} \cdot \nabla c_{i}
                        = \frac{1}{Pe}\nabla \cdot (\nabla c_{i} 
                    + z_{i} c_{i}\nabla \phi)\) &  \\
\(t_{ref}=L/U\) & \(\Lambda=\frac{\lambda}{L}\) & \(-2 \Lambda^2 \nabla^2\phi = \Sigma c_i z_i\) & \(\frac{\varepsilon}{\eta LU} \left (\frac{RT}{F}\right)^2\)\\
\(p_{ref} = \rho U^2\) & \(Re=\frac{\rho UL}{\eta}\) & \( \frac{d\vec{u}}{dt} + \vec{u}\cdot\nabla\vec{u}
                        =- \nabla p + \frac{1}{Re}\nabla^{2}\vec{u}
                            - \frac{\kappa}{2\Lambda^2} \Sigma c_i z_i\nabla \phi\)\ &  \\

\cmidrule(l){1-4} % Horizontal line spanning less than the full width of the

\(U_{ref} = D/L\) & \(Sc=\frac{\eta}{\rho D}\) & \(\frac{dc_{i}}{dt} + \vec{u} \cdot \nabla c_{i} = \nabla \cdot (\nabla c_{i} + z_{i} c_{i}\nabla \phi)\) &  \\
\(t_{ref}=L^2/D\) & \(\Lambda=\frac{\lambda}{L}\) & \(-2 \Lambda^2 \nabla^2\phi = \Sigma c_i z_i\) & \(\frac{\varepsilon}{\eta LU} \left (\frac{RT}{F}\right)^2\)\\
\(p_{ref} = \eta D/L^2\) &  & \(\frac{1}{Sc}(\frac{d\vec{u}}{dt} + \vec{u}\cdot\nabla\vec{u})
                            =-\nabla p + \nabla^{2}\vec{u}
                                - \frac{\kappa}{2\Lambda^2}\Sigma c_i z_i\nabla \phi\)\ &  \\
                                
\cmidrule(l){1-4} % Horizontal line spanning less than the full width of the

\(U_{ref} = D/L\) & \(Sc=\frac{\eta}{\rho D}\) & \(\frac{dc_{i}}{dt} + \vec{u} \cdot \nabla c_{i} = \nabla \cdot (\nabla c_{i} + z_{i} c_{i}\nabla \phi)\) &  \\
\(t_{ref}=L^2/D\) & \(\Lambda=\frac{\lambda}{L}\) & \(-2 \Lambda^2 \nabla^2\phi = \Sigma c_i z_i\) & \(\frac{\varepsilon}{\eta LU} \left (\frac{RT}{F}\right)^2\)\\
\(p_{ref} = \rho D^2/L^2\) &  & \(\frac{d\vec{u}}{dt} + \vec{u}\cdot\nabla\vec{u} =-\nabla p + Sc \: \nabla^{2}\vec{u}
                            - \frac{\kappa}{2\Lambda^2}\Sigma c_i z_i\nabla \phi\)\ &  \\
                            
\bottomrule % Bottom horizontal line
\end{tabular}
\caption{Non-dimensional forms of NS-PNP}
\label{Tab:NDTable}
\end{table}
\end{landscape}
